# Supplementary material for: DexVLG: Dexterous Vision-Language-Grasp Model at Scale
Source: arXiv:2507.02747 source file (2025-07-03)
Supplement: Supplementary file 2 [file Supp.exp_setting.tex]

\section{More Details about Benchmark and Experiment Settings}
\lidanshi{Give details of simulation benchmarks, real-world settings}
